# Supplementary material for: Evidence for magnetospheric effects on the radiation of radio pulsars
Source: arXiv:1811.12831 source file (2018-11-30)
Supplement: Supplementary file 2 [file table_appendix1.tex]

\begin{table}

\caption{A table containing high S/N pulsars which show significant phase-resolved RM variations. 
For each of these pulsars we considered the systematics uncertainty contribution that the incorrect addition of individual observations has on the shape of the RM$(\phi)$ variations.
The second column displays the time of arrival uncertainty for each pulsar, which shows the precision with which the individual observations were aligned. } 
%\citep{mhth05}}
\label{table:appendix1}
%\begin{tabular}{lllllllllllllllll}
\begin{tabular}{lr}
Pulsar name & $\sigma_{\text{ToA}}$ [$\mu$s] \\
\hline & \vspace{-3mm} \\
J0255$-$5304 &   40  \\
J0452$-$1759 &   25  \\
J0536$-$7543 &  80   \\
J0738$-$4042 &  8  \\
J0820$-$350 &  60   \\
J0835$-$4510 &  2  \\
J0837$-$4135 &  40  \\
J0908$-$4913 &  5  \\
J1001$-$5507 &  85   \\
J1057$-$5226 &  40  \\
J1243$-$6423 &  10   \\
J1326$-$5859 &  8   \\
J1453$-$6413 &  4   \\
J1456$-$6843 &  11   \\
J1559$-$4438 &  5  \\
J1701$-$3726 &  300   \\
J1731$-$4744 &  50  \\
J1751$-$4657 &  45   \\
J1820$-$0427 &  20  \\
J1824$-$1945 &  8  \\
J1900$-$600 &  40   \\
J1913$-$0440 &  40 \\
J2048$-$1616 &  180  \\

\hline
\label{tab:1}
\end{tabular}
\end{table}
